# Supplementary material for: Exact double-counting in combining the Dynamical Mean Field Theory and the Density Functional Theory
Source: arXiv:1501.03438 source file (2015-01-14)
Supplement: Supplementary file 1 [file suppl.pdf]

# Supplementary Information: Exact double-counting in combining the Dynamical Mean Field Theory and the Density Functional Theory

PACS numbers:

## DMFT PROJECTOR

The DMFT local Green's function is obtained from the total Green's function of the solid by a projection, defined by

$$G_{local}(\mathbf{r},\mathbf{r}') = \sum_{L,L'} \langle \mathbf{r}|\Phi_L\rangle \langle\Phi_L| G |\phi_{L'}\rangle \langle\phi_{L'}|\mathbf{r}'\rangle \tag{1}$$

where the the quasi-localized wave function $\langle \mathbf{r}|\Phi_L\rangle = \frac{u_l(r)}{r} Y_L(\mathbf{r})$ are the solution of the Dirac equation inside the muffin-tin sphere in the scalar relativistic approximation. The linearization energy $E_\nu$ is here chosen at the Fermi level $E_\nu = E_F$, to have very precise wave function in the vicinity of the Fermi level. In Figure 1 we plot the radial part of the wave functions $u_l(r)$ used to build the projector for $SrVO_3$, $LaVO_3$ and Cerium. In transition metal oxides we project to the $3d$ orbitals of Vanadium, and in Cerium metal we projected to Ce-$4f$ orbitals.

The projector, when written in Kohn-Sham basis, is orthonormalized locally, so that the resulting local Green's function has correct normalization, i.e., $\lim_{i\omega\to\infty} G_{local}(i\omega) = \frac{1}{i\omega} + \cdots$.

Notice that we do not remove the rest of the states from consideration, as is customary done when low energy Hubbard models are build. We just treat the above defined "correlated" states dynamically, and the rest of the states statically within LDA, hence we allow strong hybridization between "correlated" states and the itinerant states.

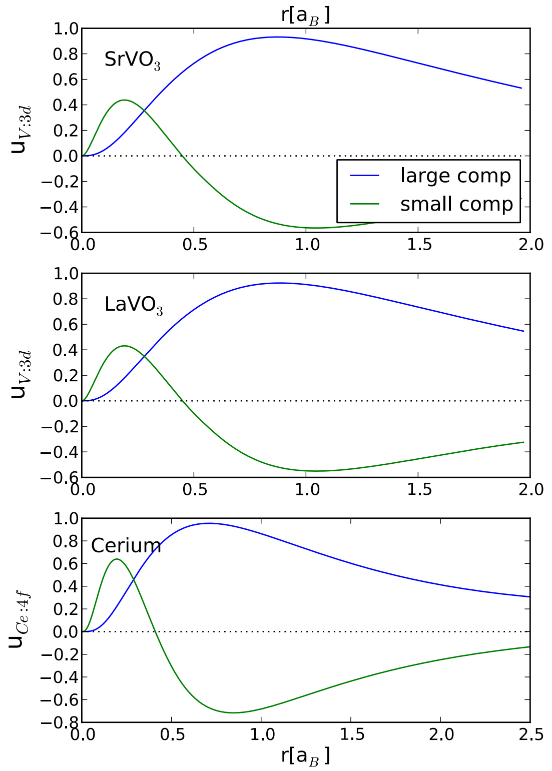


FIG. 1: The radial wave functions $u_l(r)$, which are used to build the DMFT projector and the local Green's function. We show both the large and the small component of the solution of the Dirac equation.

## SCREENED COULOMB REPULSION OF YUKAWA FORM

It is noted in the manuscript that there is a unique relationship between the inverse screening length $\lambda$ and the Hubbard interaction $U$. Moreover, Hund's coupling as well as higher order Slater integrals, are uniquely determined either from $U \equiv F^0$ or from $\lambda$. Here we derive the precise relationship between Slater integrals and screening $\lambda$.

The matrix elements of the screened Coulomb repulsion (of Yukawa form) in the orbital basis defined above are

$$U_{m_1m_2m_3m_4} = \int d^3r \int d^3r' \left(\frac{u_l(r)}{r}\right)^2 \left(\frac{u_l(r')}{r'}\right)^2 Y^*_{lm_1}(\hat{\mathbf{r}})Y_{lm_4}(\hat{\mathbf{r}})Y^*_{lm_2}(\hat{\mathbf{r}}')Y_{lm_3}(\hat{\mathbf{r}}')\frac{e^{-\lambda|\mathbf{r}-\mathbf{r}'|}}{|\mathbf{r}-\mathbf{r}'|} \tag{2}$$

There exist a well known expansion of Yukawa interaction in terms of spheric harmonics $Y_{km}$, which reads

$$\frac{e^{-\lambda|\mathbf{r}-\mathbf{r}'|}}{|\mathbf{r}-\mathbf{r}'|} = 4\pi \sum_k \frac{I_{k+1/2}(r_<)K_{k+1/2}(r_>)}{\sqrt{r_<\, r_>}} \sum_m Y^*_{km}(\hat{\mathbf{r}})Y_{km}(\hat{\mathbf{r}}') \tag{3}$$

Here $r_< = min(r, r')$, $r_> = max(r, r')$, $I$ and $K$ are modified Bessel function of the first and second kind. Inserting this expression into Eq. 2, we get

$$U_{m_1m_2m_3m_4} = \sum_k \frac{4\pi}{2k+1} \langle Y_{lm_1}|Y_{km_1-m_4}|Y_{lm_4}\rangle \langle Y_{lm_2}|Y^*_{km_3-m_2}|Y_{lm_3}\rangle$$

$$\times(2k+1)\int_0^\infty dr \int_0^\infty dr' u_l^2(r)u_l^2(r')\frac{I_{k+1/2}(\lambda r_<)K_{k+1/2}(\lambda r_>)}{\sqrt{r_<\, r_>}}. \tag{4}$$

Hence, the screened Coulomb interaction has the Slater form with the Slater integrals being

$$F^k = (2k+1)\int_0^\infty dr \int_0^\infty dr' u_l^2(r)u_l^2(r')\frac{I_{k+1/2}(\lambda r_<)K_{k+1/2}(\lambda r_>)}{\sqrt{r_<\, r_>}}. \tag{5}$$

This is a product of two one-dimensional integrals and is very easy to efficiently implement.

It is clear from Eq. 5 that $\lambda$ uniquely determines all $F^k$'s, and furthermore even one Slater integral ($F^0$) uniquely determines $\lambda$. This is because $F^k$ are monotonic functions of $\lambda$ and take the value of bare $F^k$ at $\lambda = 0$ and vanish at large $\lambda$. Hence given $F^0$, the screening length $\lambda$ is uniquely determined, and hence other higher order $F^k$ are uniquely determined as well.

## NOTE ON DERIVATION OF THE EXACT DOUBLE-COUNTING

Most of double-counting formulas were historically derived by approximating the Hubbard interaction term (defined with the help of matrix elements Eq. 2) by some static approximation, either in the atomic limit, or, in Hartree-Fock limit. Such static approximations were argued to be a good substitute for LDA treatment of the Hubbard interaction, which constitutes the double-counting term. Hence, the problem arrose becase the Hubbard model can not be solved by LDA, so that the LDA approximation for the Hubbard term could be subtracted from dynamic self-energy computed by many body method.

Here we show that if Luttinger-Ward functionals for the two approximate methods are written side-by side in the same form, the intersection of the two is evident. In other words, we can either perform the DMFT approximation on LDA functional, or, the LDA approximation on the DMFT functional, and in both cases arrive at the same term, which is counted twice.

Let's consider the lowest order term in the interaction, the Hartree term, because it can be explicitely written down. The exact Hartree term takes the form

$$E^H[\rho] = \frac{1}{2}\int d\mathbf{r}d\mathbf{r}' \frac{\rho(\mathbf{r})\rho(\mathbf{r}')}{|\mathbf{r}-\mathbf{r}'|} \tag{6}$$

In the DMFT approximation, the Hartree term is approximated by its local and screened counterpart:

$$E^H_{DMFT}[\rho] = \frac{1}{2}\int d\mathbf{r}d\mathbf{r}'(\hat{P}\rho(\mathbf{r}))(\hat{P}\rho(\mathbf{r}'))V_c^\lambda(|\mathbf{r}-\mathbf{r}'|) \tag{7}$$

Notice that when this expression is written in orbital basis, it gives exactly the Hartree term, which appears in DMFT.

The LDA implementation includes the exact Hartree term Eq. 6, and DMFT includes the approximation Eq. 7. When the two Luttinger-Ward functionals are added in LDA+DMFT, we must subtract the entire DMFT approximation for Hartree term Eq. 7, because this term was already accounted for by LDA exactly, hence no extra DMFT term is needed to this order.

Next we consider the exchange term. The exact exchange takes the following form:

$$E^X[\rho] = -\frac{1}{2}\sum_\sigma \int d\mathbf{r}d\mathbf{r}' \frac{\rho_\sigma(\mathbf{r},\mathbf{r}')\rho_\sigma(\mathbf{r}',\mathbf{r}')}{|\mathbf{r}-\mathbf{r}'|} \tag{8}$$

However, the LDA method does not take into account the exact exchange term, but it approximates it with the following approximation

$$E^X_{LDA} = -\frac{1}{2}\sum_\sigma \int d\mathbf{r}d\mathbf{r}' \rho^0_\sigma(\mathbf{r},\mathbf{r}')\rho^0_\sigma(\mathbf{r}',\mathbf{r}) V_c^{\lambda=0}(|\mathbf{r}-\mathbf{r}'|) \tag{9}$$

where $\rho^0$ is the charge density of the corresponding electron gas problem, namely,

$$\rho^0_\sigma(\mathbf{r},\mathbf{r}') = \int \frac{d^3k}{(2\pi)^3} e^{i\mathbf{k}(\mathbf{r}-\mathbf{r}')} f(\frac{k^2}{2m} - E_F) \tag{10}$$

where $f$ is the fermi function (at $T = 0$) and $E_F = (2\pi^2\rho)^{2/3}/(2m)$ .

Notice that the LDA exchange is obtained from Eq. 8 by replacing the density $\rho_\sigma(\mathbf{r},\mathbf{r}')$ of the solid by the simpler density of the electron gas problem, $\rho^0_\sigma$. The only way the real solid and electron gas problem are linked is throuh determination of $E_F$ of the corresponding electron gas problem.

The DMFT approximates the exact exchange Eq. 8 by the following truncation of variables,

$$\rho \to \hat{P}\rho \tag{11}$$

$$V_c^{\lambda=0} \to V_c^\lambda \tag{12}$$

hence the DMFT includes the following exchange term

$$E^X_{DMFT} = -\frac{1}{2}\sum_\sigma \int d\mathbf{r}d\mathbf{r}' (\hat{P}\rho_\sigma(\mathbf{r},\mathbf{r}'))(\hat{P}\rho_\sigma(\mathbf{r}',\mathbf{r}')) V_c^\lambda(|\mathbf{r}-\mathbf{r}'|) \tag{13}$$

Now, having both LDA and DMFT functionals for exchange written in the same form, Eq. 9 and Eq. 13, it becomes clear how to perform LDA approximation on DMFT functional, or, DMFT approximation on LDA functional. This is the double-counting term.

In the DMFT approximation on top of LDA functional Eq. 9, we need to replace $V_c^{\lambda=0}$ with $V_c^\lambda$ and replace $\rho$ in the electron gas fermi level EF with $\rho_{local}$. When performing LDA approximation on the DMFT functional Eq. 13, we replace real density $\hat{P}\rho$ by $\rho^0$ of electron gas, and determine the fermi level EF by the density of the solid $\hat{P}\rho = \rho_{local}$. In both cases, we arrive at the exact intersection of the two methods (for exchange term):

$$E^X_{DC} = -\frac{1}{2}\int d\mathbf{r}d\mathbf{r}' \rho^0_\sigma(\mathbf{r},\mathbf{r}')\rho^0_\sigma(\mathbf{r}',\mathbf{r}') V_c^\lambda(|\mathbf{r}-\mathbf{r}'|) \tag{14}$$

where

$$\rho^0(\mathbf{r},\mathbf{r}') = \int \frac{d^3k}{(2\pi)^3} e^{i\mathbf{k}(\mathbf{r}-\mathbf{r}')} f(\frac{k^2}{2m} - E_F) \tag{15}$$

and

$$E_F = (2\pi^2\hat{P}\rho)^{2/3}/(2m) = (2\pi^2\hat{P}\rho_{local})^{2/3}/(2m).$$

We can continue the same derivation for the correlation term. The result is easiest to derive if we perform the DMFT approximation on LDA functional. The resulting double-counting of LDA+DMFT is

$$\Phi_{DC}^{DFT+DMFT}[\rho] = E^H_{V_c^\lambda}[\hat{P}\rho] + E^{XC}_{V_c^\lambda}[\hat{P}\rho]. \tag{16}$$
